# Supplementary material for: MeshfreeFlowNet: A Physics-Constrained Deep Continuous Space-Time Super-Resolution Framework
Source: arXiv:2005.01463 source file (2020-08-21)
Supplement: Supplementary file 1 [file 8-Appendix.tex]

\onecolumn
\section*{Appendix}
Additionally, we investigate the influence that the presence of noise would have on the performance of the super-resolution task. Table \ref{table:noisydata} shows the performance of \alg for super-resolving a coarse dataset with an artificially added random Gaussian noise. Here, we add in the normalized space of the physical parameters, namely, $T$, $u$, $w$, and $p$, a random Gaussian noise with zero mean and unity standard deviation. As indicated in Table \ref{table:noisydata}, although the performance of the super-resolution framework gets slightly influenced by the noise in the dataset, it still performs reasonably well, as quantified by the physical accuracy metrics. It is worth noting that, such a good performance on a noisy dataset is achieved although the model has not been trained on noisy datasets.

\begin{table*}[h!]
\centering
\resizebox{0.8\columnwidth}{!}{
\begin{tabular}{c|ccccccccc|c}
& \multicolumn{9}{c|}{\makecell{100$\times$NMAE\\(R2)}}                                       & \multicolumn{1}{c}{} \\
\makecell{Dataset} & $E_{tot}$ & $u_{rms}$ & $\varepsilon$ & $\lambda$ & $Re_{\lambda}$ & $\tau_{\eta}$ & $\eta$ & $L$ & $T_L$ & avg. R2 \\ \hline
Clean &\makecell{0.698\\(0.9990)}    &\makecell{{0.666}\\(0.9987)}   &\makecell{{0.671}\\(0.9989)}   &\makecell{{0.554}\\(0.9983)}   &\makecell{{0.408}\\(0.9991)}   &\makecell{{0.805}\\(0.9971)}  &\makecell{{0.767}\\(0.9978)}   &\makecell{1.048\\(0.9946)}   &\makecell{{0.515}\\(0.9992)}   &0.9981                      \\ \cline{1-1}
Noisy &
       \makecell{{3.874}\\(0.9470)}&\makecell{{8.755}\\(0.8904)}&
       \makecell{{3.718}\\(0.9498)}&\makecell{{9.481}\\(0.8316)}&
       \makecell{{8.0351}\\(0.8367)}&\makecell{{10.783}\\(0.8351)}&
       \makecell{{10.234}\\(0.8584)}&\makecell{{4.582}\\(0.9440)}&
       \makecell{{5.073}\\(0.8642)}& {0.8841}                     
\end{tabular}
}
\vspace{1 pt}
\caption{For a \alg model that has been trained on one clean dataset, the super-resolution performance evaluation is respectively reported for clean and noisy coarse datasets with un-seen initial conditions. In the noisy dataset, a Gaussian noise with zero mean and unity standard deviation has been added in the normalized space of the physical parameters to the spatial coarse scale information at each time frame.}
\label{table:noisydata}
\end{table*}
